# Supplementary material for: Distributionally Robust Policy and Lyapunov-Certificate Learning
Source: arXiv:2404.03017 source file (2024-08-03)
Supplement: Supplementary file 1 [file Appendix.tex]

\section{Pointwise Distributionally Robust Formulation}
\label{sec: appendix}

As an alternative to \eqref{eq: ccp}, we can consider a pointwise probability formulation, which enforces the Lyapunov derivative condition at each state $\bfx \in \calX$ individually:
\new{
\begin{equation}
\label{eq: point_ccp}
    \bbP^*(\dot{V}(\bfx, \bfpi(\bfx), \bfxi) + \gamma \| \bfx \|  \leq 0) \geq 1-\epsilon, \; \forall \bfx \in \calX
\end{equation}
}
where $\gamma \in \bbR_{>0}$ and $\epsilon \in (0,1)$ is a user-specified risk tolerance. 
Similar to \eqref{eq: cvar_ccp}, we have a convex CVaR approximation of the chance constraint in \eqref{eq: point_ccp} as follows, 
\new{
\begin{equation}
\label{eq: point_cvar_ccp}
\begin{aligned}
     \textrm{CVaR}_{1-\epsilon}^{\mathbb{P}^*}(\dot{V}(\bfx, \bfpi(\bfx), \bfxi) + \gamma \| \bfx \|) \leq 0 , \; \; \forall \bfx \in \calX. 
\end{aligned}
\end{equation}
}
This inequality implies the satisfaction of the original chance constraint in \eqref{eq: point_ccp}.

To handle the case where the true distribution $\bbP^*$ is unknown and may shift during deployment, we can formulate a pointwise distributionally robust constraint similar to \eqref{eq: dr_clf_control_constraint}:
\new{
\begin{equation}
\begin{aligned}
\label{eq: point_dr_clf_control_constraint}
     \inf_{\bbP \in \calM_{N}^{r}}\mathbb{P}(\dot{V}(\bfx, \bfpi(\bfx), \bfxi) + \gamma \| \bfx \| \leq 0) \geq 1 - \epsilon , \; \; \forall \bfx \in \calX
\end{aligned}
\end{equation}
}

The following lemma, analogous to Lemma~\ref{lemma: dr_controller_guarantee}, characterizes the pointwise stability properties of the closed-loop system. 

\begin{lemma}[\textbf{Chance-constraint satisfaction under the true distribution}]\label{lemma: point_dr_controller_guarantee}
Assume the distribution $\bbP^*$ of $\bfxi$ in \eqref{eq: uncertain_system} is light-tailed and the Wasserstein radius $r_N(\bar{\epsilon})$ is set according to~\eqref{eq: wasserstein_r_guarantee}. If the controller $\bfpi^*(\bfx)$ and Lyapunov function $V^*(\bfx)$ pair satisfies \eqref{eq: point_dr_clf_control_constraint} with $r=r_N(\bar{\epsilon})$, then, $\forall \bfx \in \calX$, 
\begin{equation}
\label{eq: point_dr_LF_stable_guarantee}
\bbP^*(\dot{V}^*(\bfx,\bfpi^*(\bfx), \bfxi) + \gamma \| \bfx \| \leq 0) \geq (1-\epsilon)(1- \bar{\epsilon}).     
\end{equation}
\end{lemma}

Lemma~\ref{lemma: dr_controller_guarantee} demonstrates that if a pair $(V^*, \bfpi^*)$ satisfies the pointwise constraint \eqref{eq: point_dr_clf_control_constraint}, then for each $\bfx \in \calX$, the system fulfills the Lyapunov stability condition with high probability under the true distribution $\bbP^*$. 

Next, similar to Proposition~\ref{proposition: relaxed_dr_clf_constraint}, we have the following proposition for the pointwise formulation:

\new{
\begin{proposition}[\textbf{Pointwise Distributionally Robust Stability Condition}]
\label{proposition: relaxed_dr_clf_constraint_pointwise}
Let $\{\bfxi_i\}_{i \in [N]}$ be a set of samples of the uncertainty parameter $\bfxi$. Assume that the samples are indexed such that $\dot{V}(\bfx, \bfpi(\bfx), \bfxi_i) \geq \dot{V}(\bfx, \bfpi(\bfx), \bfxi_k)$, for all $1 \leq i < k \leq N$.
For $\epsilon \in (0, 1)$, let $j \in [N]$ be the unique index that satisfies $\frac{j-1}{N} - \epsilon < 0$ and $\frac{j}{N} - \epsilon \geq 0$. Then, the following condition, $\forall \bfx \in \calX$,
\begin{align}
\label{eq: point_dr_clf_constraint_relaxed}
&\frac{r}{\epsilon} \| \bfW^\top(\bfx, \bfpi(\bfx)) \nabla V(\bfx) \| + \frac{1}{N \epsilon} \sum_{i=1}^{j-1} \Big(\dot{V}(\bfx, \bfpi(\bfx), \bfxi_i) \notag \\
&- \dot{V}(\bfx, \bfpi(\bfx), \bfxi_j)\Big) + (\dot{V}(\bfx, \bfpi(\bfx), \bfxi_j) + \gamma \|\bfx\|) \leq 0 
\end{align}
is a sufficient condition for the distributionally robust stability constraint~\eqref{eq: point_dr_clf_control_constraint} to hold with the ambiguity set corresponding to the 1-Wasserstein distance. Furthermore, when $\epsilon \leq \frac{1}{N}$, the condition~\eqref{eq: dr_clf_constraint_relaxed} simplifies to: $\forall \bfx \in \calX$,
\begin{align}
\label{eq: point_dr_clf_constraint_special}
\frac{r}{\epsilon} \| \bfW^\top(\bfx, \bfpi(\bfx)) \nabla V(\bfx) \| &+ \max_{i}(\dot{V} (\bfx, \bfpi(\bfx), \bfxi_i)) \notag \\
&+ \gamma \|\bfx\| \leq 0.
\end{align}
\end{proposition}
}

Based on the pointwise formulations, similar to Sec.~\ref{sec: clf_nn_search}, we can define the following loss functions for learning a neural network pair $(V_{\bftheta_1}(\bfx), \bfpi_{\bftheta_2}(\bfx))$:
\new{
\begin{align}
\label{eq: point_dr_lf_loss}
\ell_{\text{DR}}(\bftheta) &= \frac{1}{M}\sum_{i=1}^M (\frac{r}{\epsilon} \|\bfW^\top(\bfx_i, \bfpi_{\bftheta_2}(\bfx_i)) \nabla V_{\bftheta_1}(\bfx_i)\| + \notag \\
& \quad \max_{j}(\dot{V}_{\bftheta_1}(\bfx_i, \bfpi_{\bftheta_2}(\bfx_i), \bfxi_j)) + \gamma \|\bfx_i \|)+.
\end{align}
}

\new{
The pointwise loss function in \eqref{eq: point_dr_lf_loss} is used to train the neural network Lyapunov function and controller in the pointwise distributionally robust formulation. Compared to the uniform loss function in \eqref{eq: dr_lf_loss}, the pointwise formulation is less conservative and easier to train. 
}
\new{
However, while the pointwise formulation ensures stability with high probability for each individual state, providing a formal global stability guarantee for the entire state space remains an open research question. Despite this limitation, the pointwise distributionally robust formulation offers a valuable trade-off between computational tractability and robustness to distributional shifts in the system uncertainty. It also works well for the examples in Sec.~\ref{sec: evaluation}.}
